# Supplementary material for: Investigating Advanced Reasoning of Large Language Models via Black-Box Environment Interaction
Source: arXiv:2508.19035 source file (2026-05-06)
Supplement: Supplementary file 1 [file proof.tex]

% \section{Proof for Correctness of Evaluation}\label{proof}
% In this part, we aim to prove that an incorrect reasoning path will not lead to correctness in all test samples in the proposed black-box interaction task. 
% We first define hypothesis space $\mathcal{F}_{H_T}$ as the set of all functions that are consistent with the observed interaction history $H_T$ in exploration. 
% \begin{align}
%     \mathcal{F}_{H_T} = \{g: \mathcal{X} \to \mathcal{Y} \mid \forall (x,y) \in H_T, g(x)=y \},
% \end{align}
% where $H_T = \{(x^1,y^1), \ldots, (x^T,y^T)\}$. Let $N_0 = |\mathcal{F}_{H_T}|$. $N_0 > 1$ since the exploration is non-exhaustive. We assume that $\mathcal{F}_{H_T}$ is a finite space (The proof for an infinite space can be similarly derived).
% The hidden function of black-box $f \in \mathcal{F}_{H_T}$.
% Let $P_S$ equals to the probability of model $M$'s correctness in all $K$ test samples in $\mathcal{X}_{\text{test}}$. $P_S$ can be written as the product of conditional probabilities of being correct at each test sample $x_\text{test}^k$:
% \begin{align}
%     P(S) = \prod_{k=1}^K p_k,
% \end{align}
% where $p_k$ is defined as $P(\text{correct on }x_\text{test}^k\mid \text{correct on }x_\text{test}^1,\ldots,x_\text{test}^{k-1})$.
% At the start of turn $k$, the model has a reduced hypothesis space $\mathcal{F}_{k-1} \subseteq \mathcal{F}_{H_T}$ of size $N_{k-1}$, where $\mathcal{F}_0 = \mathcal{F}_{H_T}$. The model makes a prediction $\hat{y}^k$ for the input $x_{\text{test}}^k$. $p_k$ is determined by the composition of the current hypothesis space $\mathcal{F}_{k-1}$:
% \begin{align}
%     p_k = \frac{|\{g \in \mathcal{F}_{k-1} \mid g(x_{\text{test}}^k) = f(x_{\text{test}}^k)\}|}{N_{k-1}}
% \end{align}
% If the model is correct on $x_\text{test}^k$, the next hypothesis space becomes $\mathcal{F}_k = \{g \in \mathcal{F}_{k-1} \mid g(x_{\text{test}}^k) = f(x_{\text{test}}^k)\}$, so $N_k < N_{k-1}$ unless all functions already agreed. Recall that $N_0 > 1$, this initial ambiguity implies that for some test turn $k$, the current hypothesis space $\mathcal{F}_{k-1}$ will contain functions that disagree on the output for $x_{\text{test}}^k$. So there must exist $k\in \{1, \ldots,K\}$ that subjects to $p_k < 1$. If a non-trivial amount of ambiguity exists, such that the average probability of success per turn where ambiguity exists is $\bar{p} < 1$, then $P_S$ decays exponentially with $K$:
% \begin{equation}
%     \lim_{K \to \infty} P_S \le \lim_{K \to \infty} \bar{p}^K = 0
% \end{equation}
% Reliable success requires the probability of success to be 1.
% \begin{equation}
%     P_S = 1 \iff p_k = 1, \quad \forall k \in \{1, \dots, K\}
% \end{equation}
% This condition can only be guaranteed if no ambiguity exists for any test sample, which requires the initial hypothesis space to contain only the true black-box function $f$.
% \begin{equation}
%     P_S = 1 \iff N_0 = 1
% \end{equation}
% Therefore, any model that has not fully identified the true function $f$ during exploration ($N_0 > 1$) is statistically guaranteed to fail a sufficiently large adaptive test.
% In real practice, $N_k$ is a huge number because the exploration turns are rather limited. As a result, a not very large $K$ can assure that an incorrect reasoning path will not lead to correctness in all test samples.
